# Supplementary material for: Training Video Foundation Models with NVIDIA NeMo
Source: arXiv:2503.12964 source file (2025-03-17)
Supplement: Supplementary file 1 [file appendix.tex]

% \section{Appendix}
% \subsection{Training a Custom Video Tokenizer}
% \label{sec:appendix_vae}

% Training directly on original videos or high-resolution images is often computationally prohibitive. A widely adopted approach involves encoding the original data into a latent space using a Variational Autoencoder (video tokenizer), which reduces the data size by over 100 times, thereby significantly accelerating the learning process. As shown in Fig.~\ref{sec::training}, the training process begins with a 3D causal video tokenizer to compress video inputs, enabling efficient downstream modeling and learning. Recognizing the critical role of video tokenizers, NeMo VFM offers a comprehensive toolkit that allows users to customize or fine-tune video tokenizer models to better suit their specific needs.

% \subsubsection{Customizing Tokenizer Architecture}

% NeMo VFM leverages Hugging Face Diffusers' open-source models to enable seamless video tokenizer customization. Users can modify the video tokenizer architecture by simply adjusting a few lines in the configuration JSON files. For instance, the default video tokenizer features an 8x compression ratio in the spatial dimensions of images. Users can increase the spatial reduction by adding additional encoder or decoder blocks to achieve 8x spatio reduction, thereby reducing downstream training computational requirements by up to 4x compared to the default configuration. This approach provides users with the flexibility to balance generation quality against available computational resources.

% \subsubsection{Finetuning Video Tokenizers}

% NeMo VFM supports two types of fine-tuning: 1) Fine-tuning a pretrained model using customer in-house data. 2) Fine-tuning a customized model on customer in-house data by initializing partial weights from a pretrained model. The first approach enables users to adapt an existing model to their specific data. The second approach allows customers to modify the video tokenizer architecture, enabling adjustments to the level of data compression based on their computational resources and business requirements. We also provide users the option to use multiple loss functions, including Mean Squared Error (MSE), Kullback-Leibler (K-L) divergence loss, Learned Perceptual Image Patch Similarity (LPIPS) loss, and Generative Adversarial Network (GAN) loss. 

% % Training video tokenizers can be challenging, especially if the loss terms are not well-designed. Effective video tokenizer training typically uses a Mean Squared Error (MSE) loss to measure differences between input and reconstructed images and a Kullback-Leibler (K-L) divergence loss to quantify the discrepancy between the input and reconstructed distributions. A common drawback of video tokenizers is their tendency to produce blurry reconstructions due to the Gaussian likelihood assumption, which struggles with complex image distributions. To address this, video tokenizers are often paired with Generative Adversarial Networks (GANs) to form video tokenizer-GANs, leveraging adversarial training to encourage sharper, more realistic outputs. For example, \cite{rombach2022high} introduced a Learned Perceptual Image Patch Similarity (LPIPS) loss with a GAN to stabilize video tokenizer training, enabling more realistic reconstructions. This approach is integral to our fine-tuned video tokenizer training framework, as demonstrated in Fig.\ref{fig:video tokenizer}.

% % \begin{figure}[htbp]
% % \centering
% %     \begin{subfigure}[b]{0.38\textwidth}
% %         \centering
% %         \includegraphics[width=\textwidth]{figures/vae_1.png}
% %     \end{subfigure}
% %     \hspace*{2cm}
% %     \begin{subfigure}[b]{0.38\textwidth}
% %         \centering
% %         \includegraphics[width=\textwidth]{figures/vae_2.png}
% %     \end{subfigure}
% %     \caption{Comparison of reconstructed (left) and original (right) images using a customized Variational Autoencoder (video tokenizer) fine-tuned on proprietary data.}
% %     \label{fig:video tokenizer}
% % \end{figure}
